# Supplementary material for: Biphoton engineering using modal spatial overlap on-chip
Source: arXiv:2210.16505 source file (2022-10-29)
Supplement: Supplementary file 1 [file supplemental_document.pdf]

# Biphoton engineering using modal spatial overlap on-chip: supplemental document

## 1. Effective Indices of Supermodes

We consider the coupling between two slab modes in a one-dimensional five-layer slab waveguide with two different core layers ($\mathrm{core}_1$ and $\mathrm{core}_2$), as shown in Fig. S1 (a) (Fig. 1 (a) in the main text). The effective indices ($n_{\mathrm{eff}}$) of the two isolated modes corresponding to $\mathrm{core}_1$ and $\mathrm{core}_2$ are $n_1$ and $n_2$, respectively. They have different slopes with respect to the wavelength, and intersect at the coupling wavelength $\lambda_c$. When the two core layers are separated by a finite distance, the two modes couple with each other and form a pair of symmetric and antisymmetric supermodes.

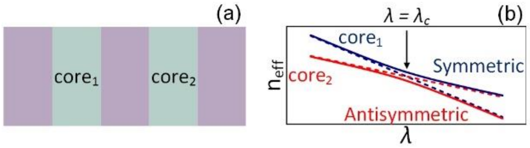


Fig. S1. (a) Schematic illustration of the five-layer slab waveguide, and (b) its $n_{\mathrm{eff}}$ of symmetric and antisymmetric supermodes. Dashed lines are the $n_{\mathrm{eff}}$ of two isolated waveguide modes.

The effective indices of the coupled symmetric ($n_+$) and antisymmetric ($n_-$) supermodes are given by [1]

$$n_\pm = \frac{1}{2}\left[(n_1 + n_2) \pm \sqrt{(n_1 - n_2)^2 + \frac{\kappa_{12}\kappa_{21}}{n_1 n_2}}\right], \tag{S1}$$

where $\kappa_{12}$ and $\kappa_{21}$ are the coupling coefficients. The difference between them is due to the different refractive index distribution of two isolated waveguides. The effective index $n_i$ ($i = 1, 2$) is a function of wavelength, and by neglecting higher-order dispersions, can be expressed as $n_i(\lambda) \approx n_i(\lambda_c) + k_i(\lambda - \lambda_c)$, with $k_i = dn_i/d\lambda$ being the slope at the coupling wavelength $\lambda_c$. Here $n_1$ and $n_2$ are equal at the coupling wavelength, i. e., $n_1(\lambda_c) = n_2(\lambda_c) = n_c$. By substituting the approximations of $n_1$ and $n_2$ given above into Eq. (S1), the $n_{\mathrm{eff}}$ of the coupled supermodes can be written as

$$n_\pm = \frac{1}{2}\left[2n_c + (k_1 + k_2)\tilde{\lambda} \pm (k_1 - k_2)\tilde{\lambda}\sqrt{1 + \varepsilon\kappa_{12}\kappa_{21}}\right], \tag{S2}$$

where $\tilde{\lambda} = \lambda - \lambda_c$, and $\varepsilon$ is a wavelength-dependent coefficient defined as

$$\varepsilon = \frac{1}{(k_1 - k_2)^2\left[k_1 k_2 \tilde{\lambda}^2 + (k_1 + k_2) n_c \tilde{\lambda} + n_c{}^2\right]\tilde{\lambda}^2}. \tag{S3}$$

The effective indices of the symmetric and antisymmetric supermodes are shown in Fig. S1 (b) (Fig. 1 (b) in the main text), using the equations derived above. In the extreme case of $\tilde{\lambda} \to \infty$, the coefficient $\varepsilon \to 0$, and the $n_{\mathrm{eff}}$ can be obtained as $n_+ \to n_2$ and $n_- \to n_1$. In the opposite extreme of $\tilde{\lambda} \to -\infty$, $\varepsilon \to 0$ as well, and the $n_{\mathrm{eff}}$ will be given by $n_+ \to n_1$ and $n_- \to n_2$ instead. Thus, moving away from $\lambda_c$, $n_{\mathrm{eff}}$ of the supermodes will asymptotically approach those of the isolated waveguide modes.

## 2. Characterization of Two-photon Quantum States

### *Two-photon States in the Asymmetrically Coupled Waveguides*

We consider SPDC in asymmetric heterogeneously coupled waveguides, as in the $\mathrm{Al}_x\mathrm{Ga}_{1-x}\mathrm{As}$-a-Si design. In this case, both symmetric (*sy*) and antisymmetric (*an*) supermodes will

participant in SPDC processes to generate photon pairs. The two-photon state of generated photon pairs can be written as

$$|\psi_{II}\rangle = \frac{1}{\sqrt{2}}\int d\omega_S d\omega_I \left[\psi_{sy}(\omega_S,\omega_I)\hat{a}^{\dagger}_{S,sy}(\omega_S)\hat{a}^{\dagger}_I(\omega_I) + \psi_{an}(\omega_S,\omega_I)\hat{a}^{\dagger}_{S,an}(\omega_S)\hat{a}^{\dagger}_I(\omega_I)\right]|0\rangle, \tag{S4}$$

where $\hat{a}^{\dagger}_{S,sy(an)}$ is the boson mode operator for the down-converted signal photons associated with the symmetric (anti-symmetric) supermode and TE polarization; $\hat{a}^{\dagger}_I$ is the operator for TM polarized idler photons in the un-coupled mode. The BWFs $\psi_{sy}(\omega_S,\omega_I)$ and $\psi_{an}(\omega_S,\omega_I)$ describe processes associated with the symmetric and anti-symmetric supermodes, respectively, and they include frequency-dependent spatial overlaps and phases due to the propagation of each mode. The operators in the supermode basis are related with operators of the uncoupled waveguide modes by

$$\hat{a}^{\dagger}_{S,sy}(\omega_S) = \frac{1}{\sqrt{2}}\left(\hat{b}^{\dagger}_1(\omega_S) + \hat{b}^{\dagger}_2(\omega_S)\right), \hat{a}^{\dagger}_{S,an}(\omega_S) = \frac{1}{\sqrt{2}}\left(\hat{b}^{\dagger}_1(\omega_S) - \hat{b}^{\dagger}_2(\omega_S)\right), \tag{S5}$$

where $\hat{b}^{\dagger}_{1,2}(\omega_S)$ are the operators of signal photon generation in two isolated waveguides. By substituting Eq. (S5) into Eq. (S4), the two-photon state can be obtained as

$$|\psi_{II}\rangle = \frac{1}{2}\int d\omega_S d\omega_I \left[\left(\psi_{sy}(\omega_S,\omega_I) + \psi_{an}(\omega_S,\omega_I)\right)\hat{b}^{\dagger}_1(\omega_S)\hat{a}^{\dagger}_I(\omega_I) + \left(\psi_{sy}(\omega_S,\omega_I) - \psi_{an}(\omega_S,\omega_I)\right)\hat{b}^{\dagger}_2(\omega_S)\hat{a}^{\dagger}_I(\omega_I)\right]|0\rangle. \tag{S6}$$

Equation (S6) tells us if one were to measure the signal photon in each individual waveguide, the probabilities of finding it would be $|\psi_{sy}(\omega_S,\omega_I) \pm \psi_{an}(\omega_S,\omega_I)|^2/4$, respectively. In this case, the signal photon will oscillate between two waveguides as it propagates, as manifested by the interference terms, with a beating length determined by the difference in the propagation constants of the two supermodes.

In our proposed technique, rather than directly collecting photons from the waveguide output, an adiabatic taper is first used to spatially separate the symmetric and anti-symmetric supermodes at all wavelengths. By spatially removing one of them (symmetric mode in the $Al_xGa_{1-x}As$-a-Si design), the remaining two-photon state becomes

$$|\psi_{II}\rangle = \int d\omega_S d\omega_I \psi_{an}(\omega_S,\omega_I)\hat{a}^{\dagger}_{S,an}(\omega_S)\hat{a}^{\dagger}_I(\omega_I)\,|0\rangle. \tag{S7}$$

As a result, not only do we remove the unwanted supermode, but also ensure that the signal photon is deterministically located in the specific waveguide by avoiding interference.

### *Polarization Entangled Photons*

The normalized two-photon state generated via type-II SPDC can be written as

$$|\psi_{II}\rangle = \frac{1}{\sqrt{2}}\int d\omega_S d\omega_I [\psi_{HV}(\omega_S,\omega_I)|\omega_S H;\omega_I V\rangle + \psi_{VH}(\omega_S,\omega_I)|\omega_S V;\omega_I H\rangle], \tag{S8}$$

where $H, V$ represent horizontal and vertical polarizations respectively, and in the main text, they are neglected for simplicity. The BWF is symmetric under the exchange of both mode indices and frequencies, i.e., $\psi_{HV}(\omega_S,\omega_I) = \psi_{VH}(\omega_I,\omega_S)$, but it does not necessarily possess any additional symmetry, i.e., $\psi_{HV}(\omega_S,\omega_I) \neq \psi_{VH}(\omega_S,\omega_I)$.

The paired photons need to be spatially separated using a dichroic mirror with a splitting frequency of $\omega_0 = \omega_P/2$, with $\omega_P$ being the central frequency of the pump. The final two-photon state can be written as

$$|\psi_{II}\rangle = \int_0^{\omega_0} d\omega_S \int_{\omega_0}^{\infty} d\omega_I [\psi_{HV}(\omega_S,\omega_I)|\omega_S H;\omega_I V\rangle + \psi_{VH}(\omega_S,\omega_I)|\omega_S V;\omega_I H\rangle]. \tag{S9}$$

According to Eq. (S9), maximal entanglement requires the paired photons to be indistinguishable in every degree of freedom except for polarization, e.g., $\psi_{HV}(\omega_S,\omega_I) = \psi_{VH}(\omega_S,\omega_I)$. However, because of the nonzero group velocity mismatch and large group

velocity dispersions, the BWF generated in $Al_xGa_{1-x}As$ waveguides is usually asymmetric. This asymmetry is manifested in both amplitude and phase of the BWF. The asymmetry in the amplitude can be removed by spectral filtering, while that in the phase can be removed by off-chip compensation that compensates for the walk-off between paired photons.

The asymmetry in the BWF can be observed in the spectral intensities of down-converted photons, i.e., $\int d\omega_I |\psi_{HV}(\omega_S, \omega_I)|^2$ for the signal and $\int d\omega_S |\psi_{HV}(\omega_S, \omega_I)|^2$ for the idler. These are equivalent to the projections of $|\psi_{HV}(\omega_S, \omega_I)|^2$ to $\omega_S$ and $\omega_I$ axes, respectively. In the special case of a CW pump, i.e., $|\alpha(\omega)|^2 = \delta(\omega - \omega_P)$, the spectral intensities are just the modular square of phase matching functions, assuming the spatial overlap does not change over wavelength.

To quantify the degree of polarization entanglement, concurrence is commonly used, which can be calculated by

$$C = 2\left|\int_0^{\omega_0} d\omega_S \int_{\omega_0}^{\infty} d\omega_I \psi_{HV}(\omega_S, \omega_I) \psi_{VH}^*(\omega_S, \omega_I)\right|. \quad \text{(S10)}$$

Maximal polarization entanglement corresponds to the maximum value of concurrence, i.e., $C = 1$, while a separable state has $C = 0$.

### *Pure Heralded Single Photons*

Photon pairs used as heralded single photons should not be correlated in frequency or any other degree of freedom. This requires that the BWF is factorable, which can be written as

$$\psi(\omega_S, \omega_I) = \psi_S(\omega_S)\psi_I(\omega_I), \quad \text{(S11)}$$

with $\psi_S(\omega_S)$ and $\psi_I(\omega_I)$ being two single-variable functions. A factorable joint spectral intensity (JSI) $|\psi(\omega_S, \omega_I)|^2$ looks like either a horizontal or vertical ellipse, or a circle.

To quantify the degree of spectral entanglement, Schmidt decomposition is performed as

$$\psi(\omega_S, \omega_I) = \sum_n \sqrt{p_n} u_n(\omega_S) v_n(\omega_I), \quad \text{(S12)}$$

where $p_n$ is the probability of obtaining the $n$-th state, with $\sum_n p_n = 1$. The degree of factorizability can be quantified by the Schmidt number given by

$$K = \frac{1}{\sum_n p_n{}^2}, \quad \text{(S13)}$$

with $K = 1$ for a separable BWF and increasing values of $K$ representing increased spectral correlations.

## 3. Separation of Symmetric and Antisymmetric Supermodes

### *Design Example Based on $Al_xGa_{1-x}As$ Waveguide*

Both symmetric and antisymmetric supermodes in the $Al_xGa_{1-x}As$-a-Si coupled ridge waveguide will take part in the pair-generation process. The $n_{\text{eff}}$ of these supermodes are shown in Fig. S2 (a). The antisymmetric supermode is required in this particular design, and the symmetric supermode is unwanted. For the isolated $Al_xGa_{1-x}As$ waveguide, the spectral intensities of down-converted photons are shown in Fig. S2 (b) (upper row of Fig. 2 (c) in the main text). The TE polarized signal spans the antisymmetric mode at $\lambda_S < \lambda_c$ and the symmetric mode at $\lambda_S > \lambda_c$. Therefore, in the coupled waveguide, signal photons are generated in both supermodes, but at different wavelength ranges.

Fig. S2 (c) and Fig. S2 (d) (the lower row of Fig. 2 (c) in the main text) show the spectral intensities of the signal in the unwanted symmetric mode and the required antisymmetric mode, respectively. The former can be removed by an adiabatic reverse taper, as shown in Fig. S3. In an adiabatic optical process, geometrical changes are sufficiently gradual, such that light that's initially in a given spatial mode maintains in that spatial mode, while the power distribution of the spatial mode will change slowly with geometry [2]. This applies to any spatial mode at any wavelength. As a result, the power in the unwanted supermode is transferred from one core to the other due to the change in spatial mode distribution, while that in the required supermode

keeps unchanged in the taper. This allows the unwanted supermode to be spatially removed when collecting the photon pairs. The general guideline for using a reverse taper or regular taper is that a regular taper removes the antisymmetric supermode while a reverse taper removes the symmetric supermode.

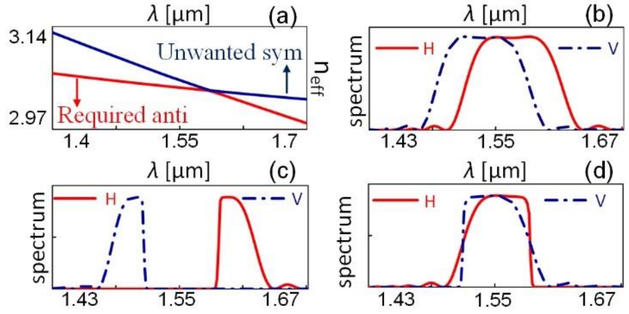


Fig. S2. (a) The $n_{\mathrm{eff}}$ of unwanted symmetric and required antisymmetric supermodes in the $Al_xGa_{1-x}$As-a-Si coupled ridge waveguide. (b) Spectral intensities of down-converted photons in the isolated $Al_xGa_{1-x}$As waveguide. (c) Spectral intensities of the unwanted symmetric and (d) required antisymmetric supermodes.

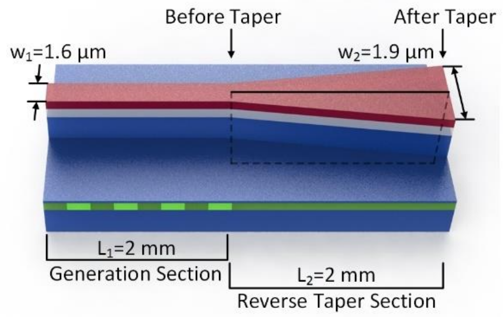


Fig. S3. Schematic of the $Al_xGa_{1-x}$As-a-Si coupled ridge waveguide with a reverse taper.

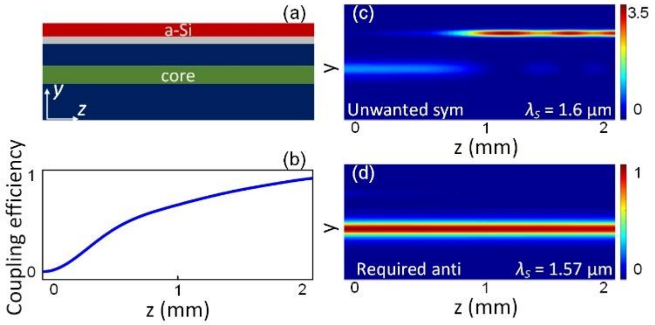


Fig. S4. (a) Schematic side-view of the reverse taper section showing all layers. (b) Dependence of the coupling efficiency on the propagation distance in the taper for unwanted supermode at $\lambda_S > \lambda_c$. (c) Simulated propagation of the unwanted supermode in the reverse taper section at $\lambda_S > \lambda_c$. (d) Simulated propagation of the required supermode in the reverse taper section at $\lambda_S < \lambda_c$.

Here we provide a specific design for the $Al_xGa_{1-x}$As-a-Si waveguide. The initial and final widths of the taper are 1.6 μm and 1.9 μm, respectively, and the length is 2 mm. A 3D FDTD fully vectorial simulation is used in the taper section to demonstrate the propagation of different

supermodes. Fig. S4 (a) shows the side view of the reverse taper section. The power in the unwanted supermode moves to the a-Si layer at $\lambda_S > \lambda_c$, and the coupling efficiency is higher than 90 %. Meanwhile, the required supermode stays in $\mathrm{Al}_x\mathrm{Ga}_{1-x}\mathrm{As}$ at $\lambda_S < \lambda_c$, as shown in Fig. S4. Thus the spatial separation of supermodes is realized on-chip. The mode beating in Fig. S4 (c) is because a small portion of light in the symmetric mode is coupled to the antisymmetric mode. This can be alleviated with a longer taper as well. The coupling efficiency can be improved with a more gradual taper. With a taper length of 3 mm, the coupling efficiency is increased to 98%. A tradeoff exists between the coupling efficiency and the overall device length.

Note that the taper is used to separate biphotons that are already engineered in the generation stage, and only serves as a complement to the whole source. In addition, based on the physics of biphoton engineering, our scheme is fundamentally different from conventional photon pair sources with post-generation on-chip spectral filters, in which the generation stages really do nothing but pair generation.

### *Design Example Based on Lithium Niobate on Insulator Waveguide*

In the example based on lithium niobate (LN), there are 3 TM polarized supermodes involved in phase matching, with their $n_{\mathrm{eff}}$ shown in Fig. S5 (a). The unwanted modes are the symmetric and antisymmetric supermodes at long and short wavelengths, respectively. Fig. S5 (b) shows the modular square of the pump envelope function ($|\alpha(\omega_S + \omega_I)|^2$). The JSIs without pump envelope, i.e., $|\phi(\omega_S, \omega_I)|^2/A(\omega_S, \omega_I)$, of the isolated waveguide and coupled waveguide with different modes are shown in Fig. S5 (c), from left to right. The corresponding final JSIs are shown in Fig. S5 (d). They show how each mode is involved in phase matching and the unwanted symmetric and antisymmetric modes at long and short wavelengths, respectively, need to be removed.

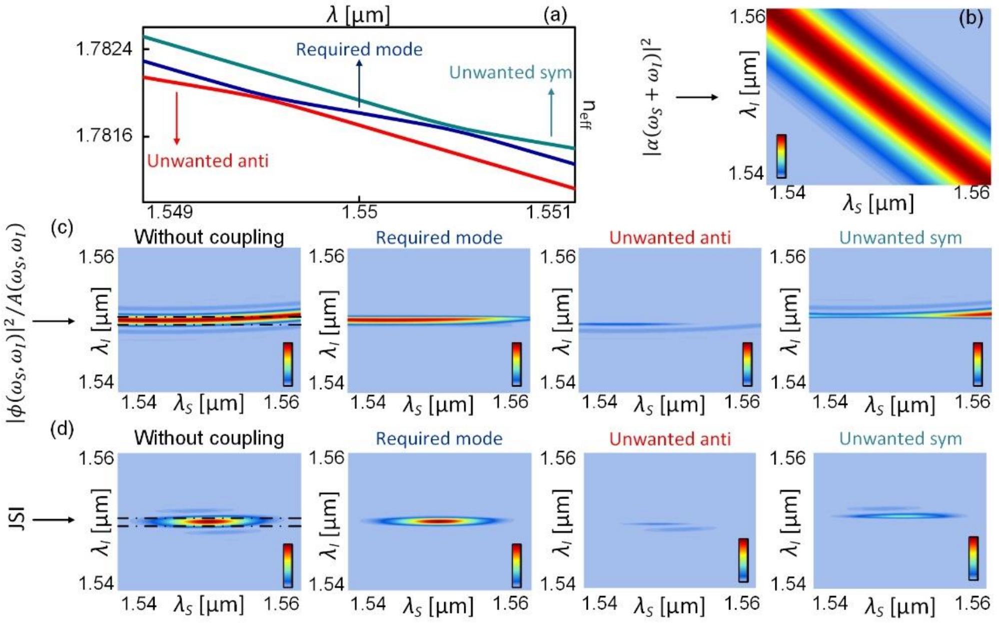


Fig. S5. (a) The $n_{\mathrm{eff}}$ of all TM supermodes involved in phase matching. (b) The JSI without pump envelope, i.e., $|\phi(\omega_S, \omega_I)|^2/A(\omega_S, \omega_I)$ of the isolated waveguide and coupled waveguide with different modes, from left to right. (c) The JSI of the isolated waveguide and coupled waveguide with different modes, from left to right.

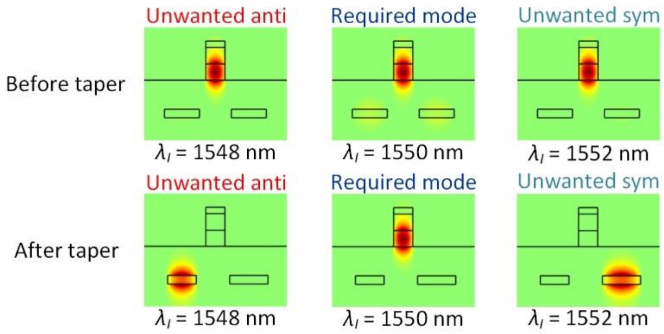


Fig. S6. The required and unwanted modal field profiles at different wavelengths before and after the tapered section.

Similarly, the unwanted supermodes can be spatially separated by adiabatic tapers. A taper is used for the antisymmetric supermode at short wavelengths, while a reverse taper is used for the symmetric supermode at long wavelengths. The specific taper designs are omitted due to substantial computational resources required, but the design principle follows the previous example. After the tapered section, the required supermode stays in LN within the required wavelength range, and the unwanted supermodes are moved to the buried $As_2Se_3$ in other wavelength ranges. In addition, after the tapers, the required supermode profile is more concentrated in the LN core, which makes it more practical for output coupling. The corresponding modal profiles are shown in Fig. S6.

## 4. Design Examples Based on Different Platforms

The strategy we propose in this work allows a broad range of materials to be considered with various host materials. The material properties required are (1) two waveguides of different materials need to have similar modal effective indices, (2) the two materials have different dispersions, and (3) they can be integrated. Therefore, more designs that utilize this technique to shape BWFs can be envisaged. In this section and the next section, we provide three additional design examples.

### *Bragg Reflection Waveguide*

A design example of practical implementation based on the Bragg Reflection Waveguide (BRW) is provided here to generate polarization entangled photons. The structure is based on the BRW reported previously [3].

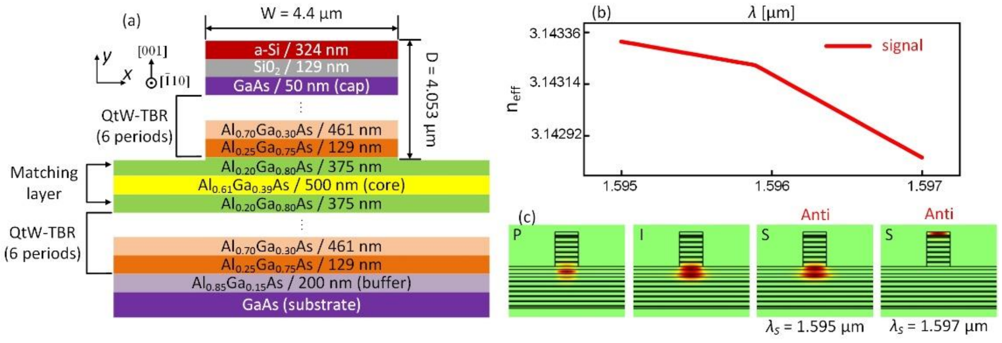


Fig. S7. (a) Schematic cross-sectional view of a coupled ridge waveguide based on BRW. (b) The $n_{\text{eff}}$ of antisymmetric TE signal mode. (c) Modal electric field profiles of pump, idler, and signal at a different wavelength. QtW-TBR: quarter-wave transverse Bragg reflector.

The corresponding design parameters are shown in Fig. S7 (a). This structure supports type-II SPDC with a TE continuous-wave (CW) pump around 775 nm and cross-polarized down-converted photons centered around 1550 nm. The signal photon is generated in the TE antisymmetric supermode while the idler is in the uncoupled TM mode. The $n_{\text{eff}}$ of signal mode is shown in Fig. S7 (b), in which the coupling wavelength is found around 1596 nm. The modal fields of the pump and idler are wavelength independent, but the location of the signal field moves from the $\text{Al}_x\text{Ga}_{1-x}\text{As}$ core to a-Si with the increase of wavelength, as shown in Fig. S7 (c). The remaining analysis is the same as the example given in the main text.

### *Dispersion Engineered LN Nanowire*

Another design based on nonlinear photonic nanowires reported in [4] is provided to generate pure heralded single photons here. The LN nanowire is dispersion engineered to achieve group velocity matching. Here two strips of buried $As_2Se_3$ are added to the original design, as shown in Fig. S8 (a). The center positions of the $As_2Se_3$ are $x_c = \pm 2$ µm and $z_c = -1.1$ µm. Again, type-II SPDC is considered, and the signal is generated in the uncoupled TE mode while idler in the TM supermode, with the $n_{\text{eff}}$ shown in Fig. S8 (b). The modal field profiles of idler at different wavelengths are shown in Fig. S8 (c). Similar to the example in the main text, this structure performs bandpass filtering to improve spectral purity.

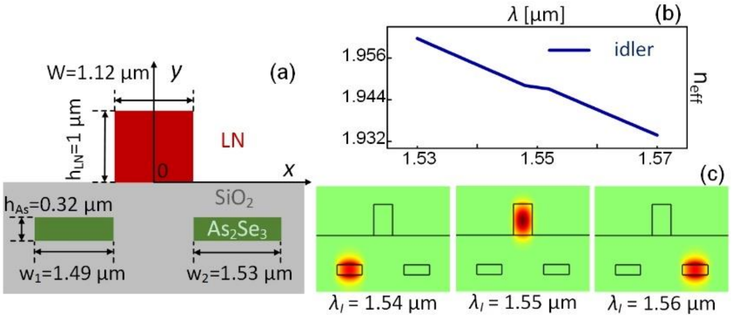


Fig. S8. (a) Schematic cross-sectional view of the coupled LN nanowire waveguide. (b) The $n_{\text{eff}}$ of TM idler mode. (c) Modal electric field profiles of idler at different wavelengths.

## 5. Design Example with Group Velocity Mismatch to Improve Spectral Purity

In the previous example as well as the example in the main text for heralded single photon generation, group velocity matching is assumed in the first place. Coupled waveguides are then constructed to perform bandpass filtering to remove the sidelobes in the JSIs. We note that the technique proposed in this work is not limited only to removing the sidelobes, but can be applied to perform narrowband filtering of BWFs in general.

The following design example is based on a conventional titanium in-diffused lithium niobate (Ti: LN) waveguide to generate pure single photons. The Ti: LN waveguide is modeled by assuming a Ti strip of 7 µm wide and 72 nm thick with a diffusion time of 6 h at a temperature of 1100 °C. Layers of $SiO_2$ and titanium dioxide ($TiO_2$) are subsequently deposited on the Ti: LN waveguide, followed by etching $TiO_2$ to form two strips. The center positions of the $TiO_2$ strips are $x_c = \pm 10$ µm. The TE polarized pump at 775 nm generates TE signal in the coupled supermode and TM idler in the uncoupled mode centered around 1550 nm using QPM. The $n_{\text{eff}}$ of TE signal is shown in Fig. S9 (b).

For the isolated Ti: LN waveguide with a length of 16 mm and a pump pulse duration of 3.5 ps, the JSI is shown in Fig. S9 (c). The corresponding Schmidt number is 4.23. For the Ti: LN-TiO2 coupled waveguide, the JSI is subject to bandpass filtering on the signal, and becomes circular, as shown in Fig. S9 (d). The Schmidt number is reduced to 1.21, showing improved spectral purity.

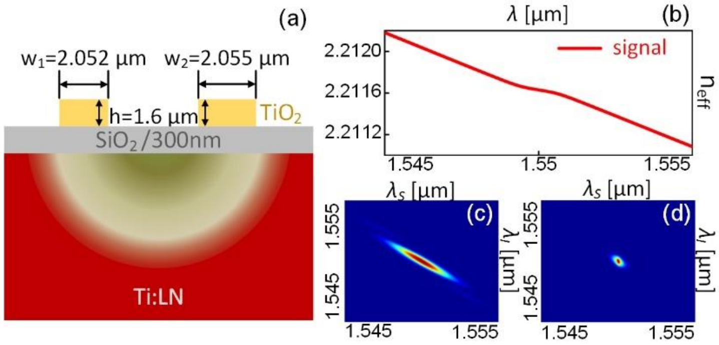


Fig. S9. (a) Schematic cross-sectional view of the Ti: LN-TiO2 coupled waveguide. (b) The $n_{\mathrm{eff}}$ of coupled TE signal mode. (c) JSI of photon pairs for the Ti: LN waveguide without coupling. (d) JSI of photon pairs for the Ti: LN-TiO2 coupled waveguide.

## References

1. J. T. Young, C. Wei, C. R. Menyuk, and J. Hu, "Mode coupling at avoided crossings in slab waveguides with comparison to optical fibers: tutorial," J. Opt. Soc. Am. B 38, F104–F114 (2021).
2. A. Milton and W. Burns, "Mode coupling in optical waveguide horns," IEEE J. Quantum Electron. 13, 828–835 (1977).
3. P. Abolghasem, J.-B. Han, D. Kang, B. J. Bijlani, and A. S. Helmy, "Monolithic photonics using second-order optical nonlinearities in multilayer-core bragg reflection waveguides," IEEE J. Sel. Top. Quantum Electron. 18, 812–825 (2012).
4. D. Kang, A. Pang, Y. Zhao, and A. S. Helmy, "Two-photon quantum state engineering in nonlinear photonic nanowires," J. Opt. Soc. Am. B 31, 1581–1589 (2014).
